# Supplementary material for: Modeling Self-Healing Behavior of Vitrimers using Molecular Dynamics with Dynamic Cross-Linking Capability
Source: arXiv:2005.02307 source file (2020-12-24)
Supplement: Supplementary file 1 [file Supplementary_Material.pdf]

# Supplementary Material: Modelling Self-Healing Behavior of Vitrimers using Molecular Dynamics with Dynamic Cross-Linking Capability

G. Singh[1] and V. Sundararaghavan[1]

[1]Department of Aerospace Engineering, University of Michigan, Ann Arbor MI 48109, U.S.A.

## Reaction in MD simulations

Figure S1 shows the schematic of a cutoff and probability-based algorithm which identifies a reaction site based on a user input template and modifies the bonding and neighboring atoms as per user specification. The bonding can have two bonding atoms only in one reaction, but the user can add any number of reactions.

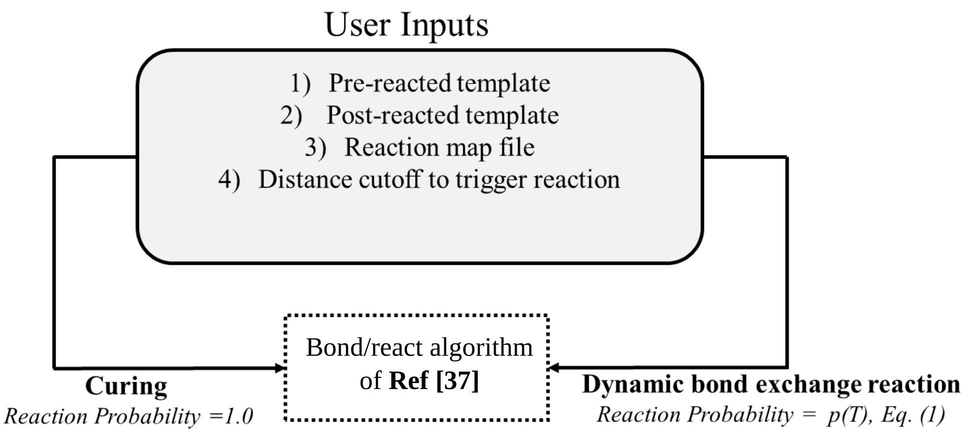


Figure S1: Using probability of the reaction in the bond/react algorithm for curing dynamic bond exchange reactions in LAMMPS

## Curing of Vitrimer

The vitrimer simulation box is filled with monomer mixture and the then the curing of the system is performed using bond/react algorithm in LAMMPS. The epoxide ring opening reaction is note modeled, instead a open ring with hydroxy group attached in the DGEBA unit is modeled direction for the curing process. To carry out the polymerization, the primary and secondary amine reactions are modeled. The pre and post reaction template for the primary and secondary reactions are shown in Figure S2(a) and S2(b), respectively.

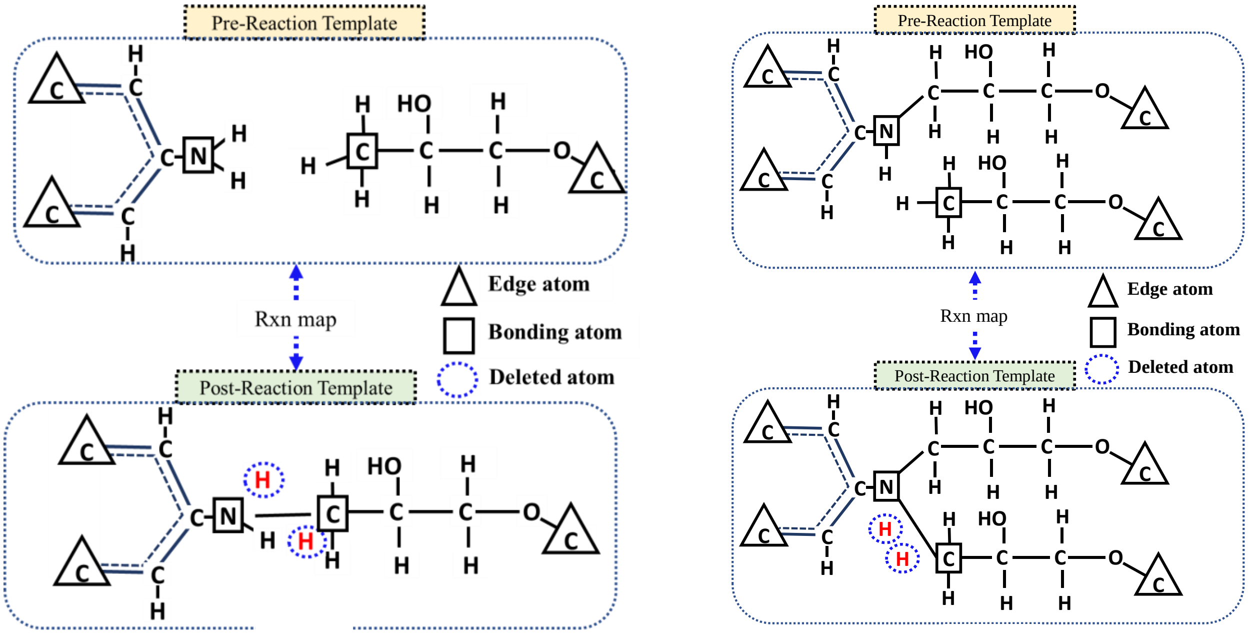


Figure S2: Reaction template for (a) primary amine and (b) secondary amine reactions in the vitrimer curing

Cross-linking of the neat vitrimer and vitrimer/CNT nanocomposite are shown in Figure S3 and S4, respectively.

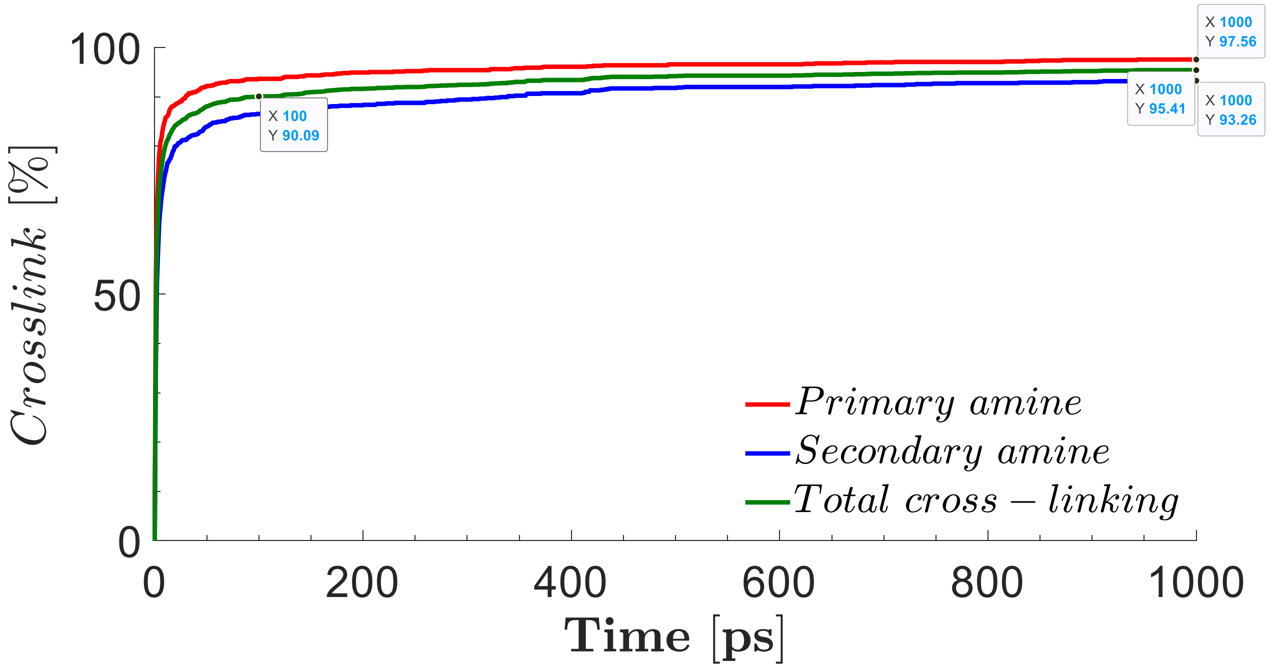


Figure S3: Crosslinking vs. time during the curing process of **neat vitrimer**

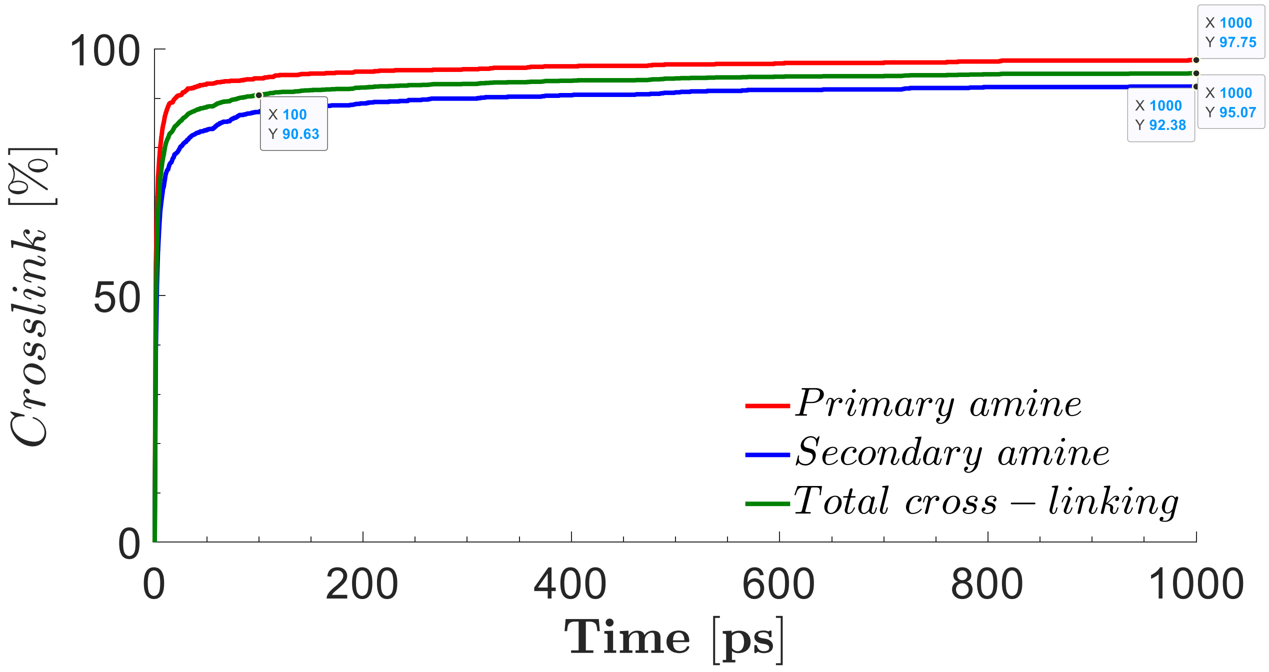


Figure S4: Crosslinking vs. time during the curing process of **vitrimer/CNT** nanocomposite

**Annealing protocol**

To obtain an equilibrated density of the cured mixture, we heat (600K) and cool (1K) at 1 bar of pressure under NPT simulations for 50ps and repeat this cycle until the density of the annealed vitrimer is converged. Converged density plot for neat vitrimer and vitrimer/CNT nanocomposite are Shown in Figure S5(a) and (b), respectively.

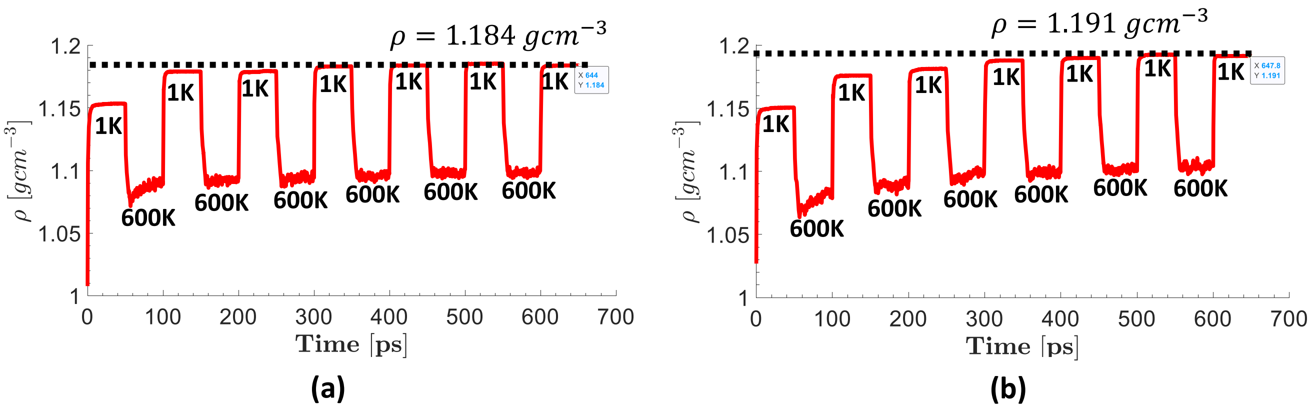


Figure S5: Density convergence of the cured (a) neat vitrimer and (b) vitrimer/CNT nancomposite under annealing

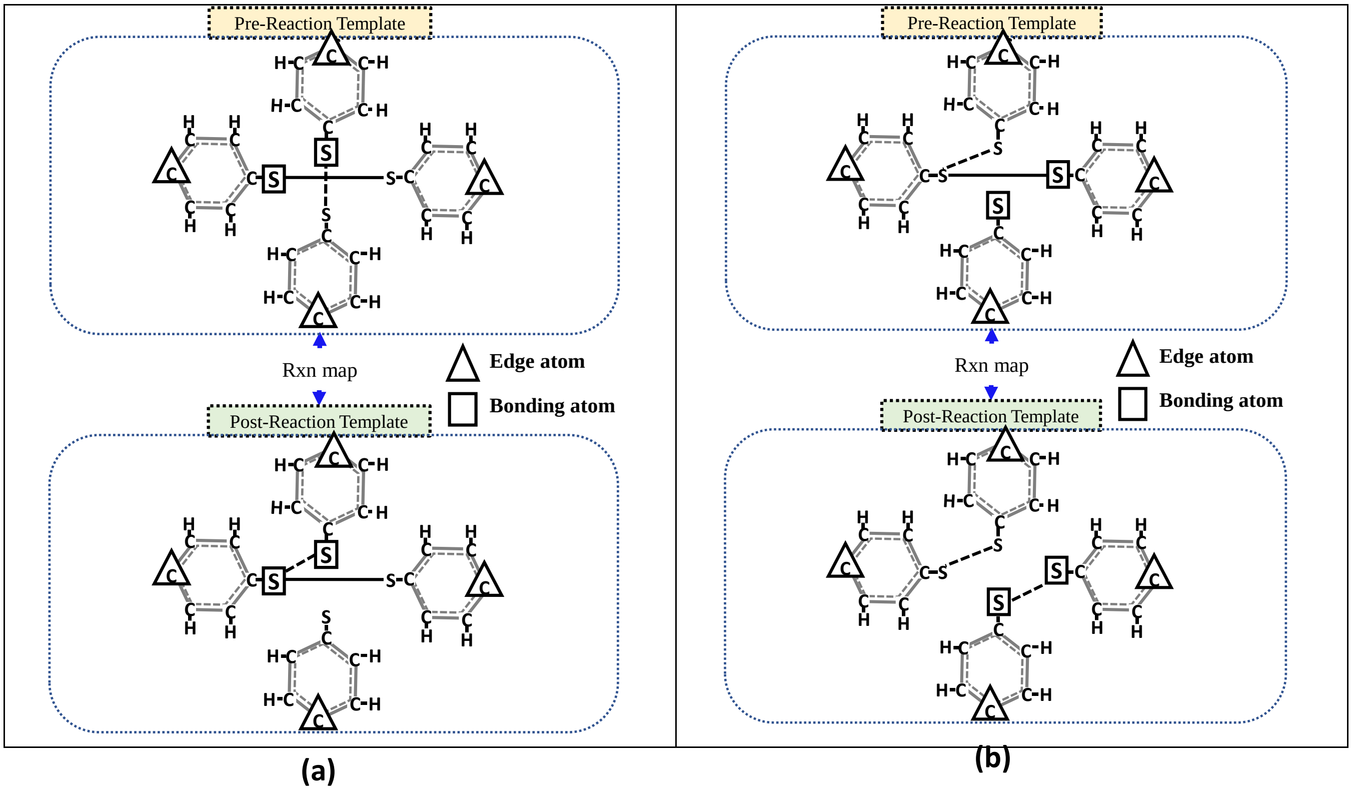


Figure S6: The dynamic bond reaction reactions modeled in two step reactions (a) breaking one S-S bond and (b) exchanging the S-S bond reaction
